# Supplementary material for: Symmetry effects on the static and dynamic properties of coupled magnetic oscillators
Source: arXiv:2204.01490 source file (2022-03-17)
Supplement: Supplementary file 1 [file SI.pdf]

# Symmetry effects on the static and dynamic properties of coupled magnetic oscillators

## Supplementary Information

### 1 FMR experimental set-up:

Figure 1(a) shows a diagram of the ferromagnetic resonance (FMR) experimental set-up. The sample is placed in a uniform external magnetic field generated by an electromagnet, which can be rotated in the plane of the device. MW current is generated by a MW source (modulated by a quasi-DC signal from a function generator) and is used to excite FMR via current-induced torques. The precessional motion of the magnetisation at resonance induces oscillations of the magneto-resistance. When multiplied by the MW current the oscillating resistance gives rise to a rectified (quasi-)DC voltage that is detected through a bias tee by a lock-in amplifier (Figure 1(a)) locked at the modulation frequency of the function generator. A more detailed description of the measurement technique is provided at ref. [1].

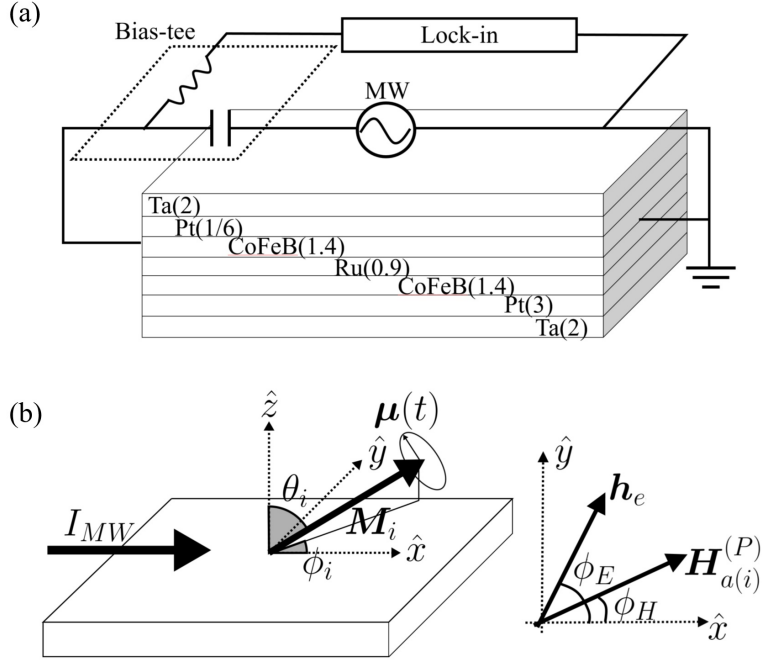

Figure 1: (a) Diagram of the experimental set-up used to measure FMR modes in the SAF structures (all thicknesses in brackets are in nm). (b) Definition of the directions. The static equilibrium magnetisation of layer  $i$ ,  $\mathbf{M}_i$ , lies at angle  $\phi_i$  to the x-axis, and  $\theta_i$  to the z-axis. When subject to an oscillating magnetic field, it oscillates about  $\mathbf{M}_i$  with instantaneous displacement vector  $\boldsymbol{\mu}(t)$ . In addition to the oscillating field, the magnetisation is subject to a static external field  $\mathbf{h}_e$ , at angle  $\phi_H$  to the x-axis, and a uni-axial anisotropy field  $\mathbf{H}_{a(i)}^{(P)}$ , at angle  $\phi_E$  to the x-axis.

## 2 Single layer characterisation:

Here we report FMR measurements carried on a single CoFeB layer, grown in the structure Ta[2]/Pt[3]/CoFeB[1.4]/Ru[0.9]/Ta[2] (all thickness in nm) by using the same growth conditions used for the growth of the SAF. The only purpose of these measurements is to characterise the magnetic anisotropy of the ferromagnet, and verify the presence of an in-plane easy axis in the direction of the magnetic field applied during growth. In the SAF structure, we can assume similar anisotropy terms for the bottom CoFeB layer.

The dynamics of a single magnetic layer subject to a microwave effective field  $\delta \mathbf{h} e^{i\omega t}$  are described by the Landau-Lifshitz-Gilbert (LLG) equation [2, 3] :

$$\frac{\partial \mathbf{m}}{\partial t} = -\gamma \mu_0 \mathbf{m} \times (\mathbf{H}_{eff} + \delta \mathbf{h} e^{i\omega t}) + \alpha \mathbf{m} \times \frac{\partial \mathbf{m}}{\partial t} \quad (1)$$

where  $\mathbf{m}$  is the normalised magnetisation vector, which is split into a static component  $\mathbf{M}$  and a transverse oscillating component  $\delta \mathbf{m}$ ,  $\mathbf{m}(t) = \mathbf{M} + \delta \mathbf{m} e^{i\omega t}$  (Figure 1(b)). The microwave field contains contributions from the field-like torque and Orested field, which lie in-plane, and the antidamping torque, which corresponds to an oscillating field in the z-direction [1]. The effective field  $\mathbf{H}_{eff}$  includes contributions from the external field  $\mathbf{h}_e$ , at an angle  $\phi_H$  with respect to the current direction (x-axis), the demagnetisation field, an in-plane uni-axial anisotropy with effective field strength  $H_a^{(P)}$  at an angle  $\phi_E$  to the x-axis, and an out of plane uni-axial anisotropy with strength  $H_a^{(N)}$ :

$$\mathbf{H}_{eff} = \mathbf{h}_e - M_s \hat{\mathbf{z}} + \hat{\mathbf{H}}_a^{(P)} (\mathbf{m} \cdot \mathbf{H}_a^{(P)}) + \hat{\mathbf{H}}_a^{(N)} (\mathbf{m} \cdot \mathbf{H}_a^{(N)}) \quad (2)$$

By linearising (1) in the zero damping limit ( $\alpha = 0$ ) we obtain the Kittel formula [4, 5]:

$$\omega/\gamma = \sqrt{(B_{res} + \mu_0 H_1)(B_{res} + \mu_0 H_2)} \quad (3)$$

$\omega = 2\pi\nu$ , where  $\nu$  is the frequency of the applied MW current,  $\gamma$  the gyromagnetic ratio for a free electron,  $B_{res}$  is the value of the external magnetic field at which the resonance occurs,  $H_1 = M_s - H_a^{(N)} + H_a^{(P)} \cos^2(\phi_H - \phi_E)$  and  $H_2 = H_a^{(P)} \cos(2(\phi_H - \phi_E))$ . Figure 2 shows the frequency dependence of  $B_{res}$  when the external field is applied along the hard-axis, i.e.  $\phi_E - \phi_H = \pi/2$ :

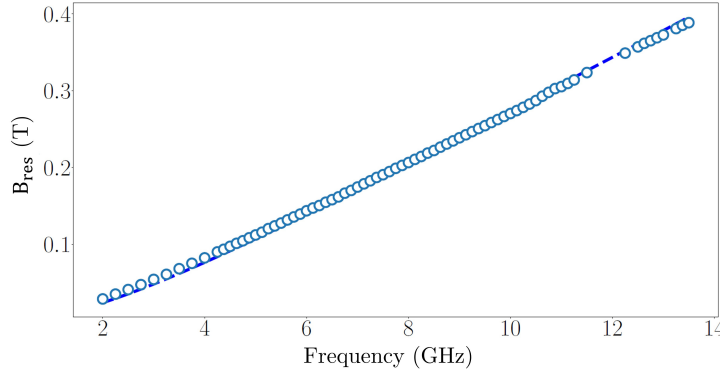

Figure 2: Dependence of the resonance field on microwave frequency. The dashed line represents a fitting obtained with Kittel formula.

By fitting the frequency dependence of  $B_{res}$  with equation (3), keeping the direction  $\phi_H$  fixed, we find the effective magnetisation of CoFeB  $M_s^{eff} = M_s - H_a^{(N)} = 211 \pm 2$  mT. This is substantially reduced compared to the bulk magnetisation of CoFeB ( $\approx 1500$  mT [6]), indicative of a significant out-of-plane anisotropy.

The strength of the in-plane uni-axial anisotropy field is found by fitting with equation (3)  $B_{res}$  vs.  $\phi_H$ , for a fixed value of  $\omega$  (Figure 3). From the fitting we obtain a field strength of  $\mu_0 H_a^{(P)} = 3.17 \pm 0.12$  mT at  $45^\circ$  with respect to the x-axis.

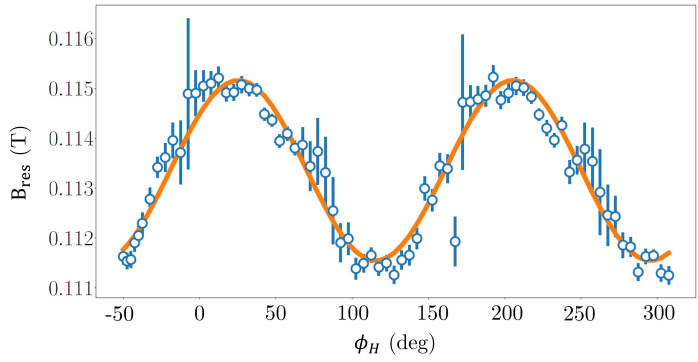

Figure 3: Value of the resonance field for a fixed value of the MW current frequency at different in-plane orientations of the field. The fitting with Kittel formula (continuous orange line) allows extracting the value of the in-plane anisotropy field  $H_a^{(P)}$ .

### 3 Static theory:

In the main article it was shown that if a symmetry operation commutes with the set of operators  $\mathbf{\Lambda}^{ij}$ , describing the effective field in layer  $i$  due to the magnetisation of layer  $j$ ,  $\mathbf{H}_{eff}^i = \mathbf{\Lambda}^{ij} \mathbf{M}_j$ , then new symmetry-transformed solutions can be constructed from previously known solutions. Here we list these operators explicitly. Most of these operators are linear, and hence will be described by matrices. The only exception of the terms we consider is the biquadratic exchange field, which has an additional  $\mathbf{m}_A \cdot \mathbf{m}_B$  factor, where  $\mathbf{m}_A$  and  $\mathbf{m}_B$  are the magnetisations of the two coupled magnets of the SAF. However, as this term is invariant under any orthogonal transformation  $\mathbf{m}_i \rightarrow R\mathbf{m}_i$ , the commutation relation can still be treated as a matrix commutation relation.

A uni-axial field in layer  $i$  can be expressed by the matrix with components:

$$(\mathbf{\Lambda}_{ani}^{ii})_{jk} = \frac{2K^{(i)}}{\mu_0 M_{si}^2} n_j^{(i)} n_k^{(i)} \quad (4)$$

where  $n_j^{(i)}$  is the  $j^{th}$  component of the unit vector in the direction of the easy axis in layer  $i$ , and  $K^{(i)}$  is the anisotropy constant that parametrises the strength of the anisotropy ( $H_a^{(i)} = 2K^{(i)}/\mu_0 M_s$ ). We include contributions from the in-plane anisotropy  $\mathbf{\Lambda}_{ani(p)}^{ii}$  and out of plane anisotropy  $\mathbf{\Lambda}_{ani(n)}^{ii}$ , where  $\mathbf{p} = (1, 1, 0)$  and  $\mathbf{n} = (0, 0, 1)$ .

The demagnetisation fields are expressed using the demagnetisation tensor of Newell et al. [7],  $\mathbf{N}^{ij}$ , as  $\mathbf{H}_{demag}^i = \mathbf{N}^{ij} \mathbf{m}_j$ .  $\mathbf{N}^{ij}$  represents the demagnetisation field in layer  $i$  due to layer  $j$ .

The demagnetisation tensor of a square bar is defined by:

$$\mathbf{N}^{ii} = \begin{bmatrix} \delta^{(i)} & 0 & 0 \\ 0 & \delta^{(i)} & 0 \\ 0 & 0 & 1 - 2\delta^{(i)} \end{bmatrix} \quad (5)$$

$$\mathbf{N}^{ij} = \begin{bmatrix} \lambda^{(ij)} & 0 & 0 \\ 0 & \lambda^{(ij)} & 0 \\ 0 & 0 & -2\lambda^{(ij)} \end{bmatrix} \quad i \neq j \quad (6)$$

in the thin-film limit  $\delta \ll 1$ . The bilinear exchange field takes the form:

$$(\mathbf{\Lambda}_{ex1}^{ij})_{kl} = \frac{-JA}{\mu_0 M_{sA} M_{sB} t_i} \delta_{kl} \quad (7)$$

Where  $J$  is the exchange constant, and  $t_i$  the thickness of layer  $i$ . A positive  $J$  corresponds to anti-ferromagnetic ordering. The biquadratic term is identical except for an additional factor of  $\mathbf{m}_A \cdot \mathbf{m}_B$ . As suggested above, when considering the commutation relations we can treat it as a matrix with components:

$$(\mathbf{\Lambda}_{ex2}^{ij})_{kl} = \frac{-2J_2}{\mu_0 M_{sA} M_{sB} t_i} \mathbf{m}_A \cdot \mathbf{m}_B \delta_{kl} \quad (8)$$

Positive  $J_2$  favours a perpendicular orientation between  $\mathbf{m}_A$  and  $\mathbf{m}_B$ . We can therefore construct the operators  $\Lambda^{ij}$  as follows:

$$\Lambda^{ii} = \Lambda_{ani(p)}^{ii} + \Lambda_{ani(n)}^{ii} - \mathbf{N}^{ii} \quad (9)$$

$$\Lambda^{ij} = \Lambda_{ex1}^{ij} + \Lambda_{ex2}^{ij} - \mathbf{N}^{ij} \quad (10)$$

It is straightforward to see that the matrix representing a reflection in the plane containing the easy/hard axis commutes with all of these operators.

### 3.1 Non-uniform magnetisation:

In this section we generalise the considerations that we make in the previous paragraph, which are at the basis of our magnetoresistance symmetry analysis, to the case in which the magnetisation has a spatial dependence. In this case Brown's equation must be satisfied at all points in space, i.e.  $\mathbf{H}_{eff}^i(\mathbf{x}) \times \mathbf{m}_i(\mathbf{x}) = 0$ . If  $R$  is a symmetry operation of the device and  $\mathbf{m}_i(\mathbf{x})$  is a solution of Brown's equation for an external field  $\mathbf{h}_e^i(\mathbf{x})$ , then so too must be  $\mathbf{m}'_i(\mathbf{x}) = R\mathbf{m}_i(R^{-1}\mathbf{x})$  for  $\mathbf{h}_e^{i'}(\mathbf{x}) = R\mathbf{h}_e^i(R^{-1}\mathbf{x})$ . Fields that depend only on the local magnetisation then transform as:

$$\mathbf{H}_{local}^{i'}(R\mathbf{x}) = R\mathbf{H}_{local}^i(\mathbf{x}) \quad (11)$$

We require the same transformation law for non-local effective fields also. The only non-local field we consider is the demagnetisation field, which in layer  $i$  at the position  $\mathbf{x}$  is given by the operator equation:

$$\mathbf{H}_{demag}^i(\mathbf{x}) = \Lambda_{demag}^{ij}(\mathbf{x})[\mathbf{m}_j(\mathbf{x})] = \int_{V_j} d\mathbf{x}' \mathbf{N}^{ij}(\mathbf{x} - \mathbf{x}') \cdot \mathbf{m}_j(\mathbf{x}') \quad (12)$$

where the integral runs over the volume of magnetic layer  $j$ . Using the ansatz  $\mathbf{m}'_j(\mathbf{x}) = R\mathbf{m}_j(R^{-1}\mathbf{x})$ , the effect field transforms as:

$$\mathbf{H}_{demag}^{i'}(R\mathbf{x}) = \int_{V_j} d\mathbf{x}' \mathbf{N}^{ij}(R\mathbf{x} - \mathbf{x}') \cdot R\mathbf{m}_j(R^{-1}\mathbf{x}') = \det R \int_{R(V_j)} d\mathbf{x}' \mathbf{N}^{ij}(R(\mathbf{x} - \mathbf{x}')) \cdot R\mathbf{m}(\mathbf{x}') \quad (13)$$

In the case considered in this report of reflection symmetry along the diagonal of a square bar, the -1 from  $\det R$  cancels with the sign change from the change in limits, and, using the transformation properties of the demagnetisation tensor [7], in particular by considering which components are even/odd under reflection in the spatial arguments, we obtain  $\mathbf{N}^{ij}(R(\mathbf{x} - \mathbf{x}'))R = R\mathbf{N}(\mathbf{x} - \mathbf{x}')$ . Hence  $\mathbf{H}_{demag}^{i'}(R\mathbf{x}) = R\mathbf{H}_{demag}^i(\mathbf{x})$ . Consequently:

$$\mathbf{H}_{eff}^{i'}(R\mathbf{x}) \times \mathbf{m}'_i(R\mathbf{x}) = (R\mathbf{H}_{eff}^i(\mathbf{x})) \times (R\mathbf{m}_i(\mathbf{x})) = \mathbf{0} \quad (14)$$

For all  $\mathbf{x}$  as required.

## 4 Dynamic theory:

The magnetisation dynamics of a series of coupled ferromagnetic oscillators can be modelled by the LLG equation:

$$\frac{d\mathbf{m}_i}{dt} = -\gamma\mathbf{m}_i \times \mathbf{H}_{eff}^i + \alpha_i\mathbf{m}_i \times \frac{d\mathbf{m}_i}{dt} \quad (15)$$

where  $\mathbf{m}_i$  is the (normalised) magnetisation of the  $i^{th}$  magnetic moment,  $\mathbf{H}_{eff}^i$  is the effective field it experiences, and  $\alpha_i$  is the Gilbert damping. From here on we will focus on the case of two coupled magnetic oscillators where the equilibrium magnetisations lie entirely in-plane, i.e.  $\theta_i = \theta_j = \pi/2$ , but this derivation is easily extended to an arbitrary number of magnetisations at arbitrary orientations [8]. We assume a solution of the form  $\mathbf{m}_i = \mathbf{M}_i + \boldsymbol{\mu}_i e^{i\omega_\mu t}$ .  $\mathbf{M}_i$  is the equilibrium magnetisation vector and  $\boldsymbol{\mu}_i$  oscillates in a plane transverse to  $\mathbf{M}_i$  with frequency  $\omega_\mu$ . In spherical coordinates  $\boldsymbol{\mu}_i$  is given by  $\boldsymbol{\mu}_i = \mu_{i\theta}\hat{\mathbf{e}}_\theta + \mu_{i\phi}\hat{\mathbf{e}}_\phi$ , where  $\hat{\mathbf{e}}_\theta$  and  $\hat{\mathbf{e}}_\phi$  are the usual unit vectors in the  $\theta$  and  $\phi$  directions.

To derive a linearised equation for the dynamics of the magnetisation, we follow the procedure of Smit and Beljers [9], the logic of which is straightforwardly illustrated in the case of a single layer, and can then be extended to the multi-layer case. The effective field is defined as the derivative of the free energy,  $U$ , with respect to the magnetisation directions and volume. Taylor expanding the magnetisation about its equilibrium direction in the usual way (noting that by definition of the equilibrium direction, all first derivatives vanish):

$$U = U_0 + \frac{1}{2} \boldsymbol{\mu}^\dagger H \boldsymbol{\mu} \quad (16)$$

Where  $\boldsymbol{\mu}$  is a small displacement,  $U_0$  is the energy at equilibrium, and  $H$  is the Hessian of  $U$ . From the definition of  $\mathbf{H}_{eff}$  we obtain:

$$\mathbf{H}_{eff} = \frac{1}{\mu_0 M_s V} H \boldsymbol{\mu} \quad (17)$$

Substituting this into the LLG equation (15) with  $\alpha = 0$  we obtain, to first order in  $\boldsymbol{\mu}$ :

$$i\omega_\mu \boldsymbol{\mu} = -\gamma \mathbf{M}_i \times \frac{1}{\mu_0 M_s V} H \boldsymbol{\mu} \quad (18)$$

Noting that  $\mathbf{M}_i$  is a unit vector in the radial direction, the cross product in (18) can be replaced by a matrix of the form  $\begin{bmatrix} 0 & -1 \\ 1 & 0 \end{bmatrix}$ . Taking the resultant matrix onto the other side, we arrive at a final form:

$$-\omega_\mu \mathcal{I} \boldsymbol{\mu} = \gamma H \boldsymbol{\mu} \quad (19)$$

Where:

$$\mathcal{I} = \mu_0 \begin{pmatrix} 0 & -iM_s V \\ iM_s V & 0 \end{pmatrix} \quad (20)$$

It is straightforward to extend this to the case of a two-layer (and higher) device with the replacement of  $H$  with the appropriate Hessian and  $\mathcal{I}$  with [8]:

$$\mathcal{I} = \mu_0 \begin{pmatrix} 0 & -iM_{sA}V_A & 0 & 0 \\ iM_{sA}V_A & 0 & 0 & 0 \\ 0 & 0 & 0 & -iM_{sB}V_B \\ 0 & 0 & iM_{sB}V_B & 0 \end{pmatrix} \quad (21)$$

where  $\boldsymbol{\mu}$  is the 4-component vector  $\boldsymbol{\mu} = (\boldsymbol{\mu}_A, \boldsymbol{\mu}_B) = (\mu_{A\theta}, \mu_{A\phi}, \mu_{B\theta}, \mu_{B\phi})$ . In this notation, definition of the oscillating effective field is given by:

$$\begin{bmatrix} h_{A\theta} \\ h_{A\phi} \\ h_{B\theta} \\ h_{B\phi} \end{bmatrix} = \begin{bmatrix} 1/M_{sA}V_A & 0 & 0 & 0 \\ 0 & 1/M_{sA}V_A & 0 & 0 \\ 0 & 0 & 1/M_{sB}V_B & 0 \\ 0 & 0 & 0 & 1/M_{sB}V_B \end{bmatrix} \begin{bmatrix} H_{AA}^{\theta\theta} & H_{AA}^{\theta\phi} & H_{AB}^{\theta\theta} & H_{AB}^{\theta\phi} \\ H_{AA}^{\phi\theta} & H_{AA}^{\phi\phi} & H_{AB}^{\phi\theta} & H_{AB}^{\phi\phi} \\ H_{BA}^{\theta\theta} & H_{BA}^{\theta\phi} & H_{BB}^{\theta\theta} & H_{BB}^{\theta\phi} \\ H_{BA}^{\phi\theta} & H_{BA}^{\phi\phi} & H_{BB}^{\phi\theta} & H_{BB}^{\phi\phi} \end{bmatrix} \begin{bmatrix} \mu_{A\theta} \\ \mu_{A\phi} \\ \mu_{B\theta} \\ \mu_{B\phi} \end{bmatrix} \quad (22)$$

Here, the component  $H_{AB}^{\theta\phi}$  for instance represents the second derivative with respect to  $\theta_A$  and  $\phi_B$  of the energy.  $M_{si}$  and  $V_i$  are respectively the saturation magnetisation and volume of magnetic layer  $i$ . The second matrix on the right is the Hessian of the energy density. Strictly, it is the curvature of the free energy density that enters into the LLG equation, but at equilibrium, where first derivatives vanish, this is equivalent to the Hessian and is denoted by  $H$  in (21).

To numerically model the resonance modes of a SAF, we find the eigenvalues of the linearised LLG equation (21) numerically. We model SAFs as having an effective field with contributions from external field, exchange fields, demagnetisation fields, and uni-axial fields. This results in a total energy of the system given by:

$$U = U_e + U_{ex} + U_{demag} + U_{ani}^A + U_{ani}^B \quad (23)$$

where  $U_e$  is the energy of the external field,  $U_{ex}$  the exchange field energy,  $U_{demag}$  the energy due to demagnetisation interactions, and  $U_{ani}^i$  the energy from uni-axial anisotropy in layer  $i$ . These terms can be written explicitly as:

$$U_e = -\mu_0 \mathbf{h}_e \cdot (\mathbf{m}_A M_{sA} V_A + \mathbf{m}_B M_{sB} V_B) \quad (24)$$

where  $\mathbf{h}_e$  is the external field, which lies in-plane at an angle  $\phi_H$  to the x-axis (Figure 1(b)).

$$U_{demag} = \frac{\mu_0 V_A}{2} M_{sA}^2 \mathbf{m}_A \cdot \mathbf{N}^{AA} \mathbf{m}_A + \frac{\mu_0 V_B}{2} M_{sB}^2 \mathbf{m}_B \cdot \mathbf{N}^{BB} \mathbf{m}_B + \frac{\mu_0 V_A}{2} M_{sA} M_{sB} \mathbf{m}_A \cdot \mathbf{N}^{AB} \mathbf{m}_B + \frac{\mu_0 V_B}{2} M_{sA} M_{sB} \mathbf{m}_B \cdot \mathbf{N}^{BA} \mathbf{m}_A \quad (25)$$

here  $\mathbf{N}^{ij}$  is the matrix that describes the demagnetisation field in layer  $i$  due to the magnetic moment in layer  $j$  as defined in (5) and (6). If we take the volumes  $V_A$  and  $V_B$  to be equal  $V_A = V_B = V$ ,  $\delta^A = \delta^B = \delta$ , and  $\mathbf{N}^{AB} = \mathbf{N}^{BA} = \text{diag}(\lambda, \lambda, -2\lambda)$ . In calculating the demagnetisation tensors we have assumed dimensions of  $5\mu\text{m} \times 5\mu\text{m} \times 1.4\text{nm}$  for both layers and a separation of  $0.9\text{nm}$ .

$$U_{ex} = J A \mathbf{m}_A \cdot \mathbf{m}_B + J_2 A (\mathbf{m}_A \cdot \mathbf{m}_B)^2 \quad (26)$$

$J$  and  $J_2$  are the exchange constants for the bilinear and biquadratic exchange fields, while  $A$  is the surface area of the bar.

$$U_{ani}^i = -\frac{\mu_0 V_i}{2} M_{si} H_{a(i)}^{(P)} \left( \mathbf{m}_i \cdot \hat{\mathbf{H}}_{a(i)}^{(P)} \right)^2 - \frac{\mu_0 V_i}{2} M_{si} H_{a(i)}^{(N)} \left( \mathbf{m}_i \cdot \hat{\mathbf{H}}_{a(i)}^{(N)} \right)^2 \quad (27)$$

$\mathbf{H}_{a(i)}^{(P)} = H_{a(i)}^{(P)} \hat{\mathbf{H}}_{a(i)}^{(P)}$  is the strength and direction of the in-plane anisotropy in layer  $i$  at angle  $\phi_E$  to the x-direction (see Figure 1(b)), and likewise  $\mathbf{H}_{a(i)}^{(N)} = H_{a(i)}^{(N)} \hat{\mathbf{H}}_{a(i)}^{(N)}$  is the strength and direction of the out of plane anisotropy in layer  $i$ . We calculate the matrix elements of the Hessian, defined in (22), from the energy given by (24)-(27):

$$\begin{aligned} \frac{1}{M_{si} V} H_{ii}^{\theta\theta} &= h_e \cos(\phi_i - \phi_H) - M_{sj} \lambda \cos(\phi_i - \phi_j) + M_{si} (1 - \delta) \\ &\quad - H_{a(i)}^{(N)} + H_{a(i)}^{(P)} \cos^2(\phi_i - \phi_E) - H_{E(i)}^{(1)} \cos(\phi_i - \phi_j) - H_{E(i)}^{(2)} \cos^2(\phi_i - \phi_j) \end{aligned} \quad (28)$$

$$\begin{aligned} \frac{1}{M_{si} V} H_{ii}^{\phi\phi} &= h_e \cos(\phi_i - \phi_H) - M_{sj} \lambda \cos(\phi_i - \phi_j) + H_{a(i)}^{(P)} \cos(2(\phi_i - \phi_E)) - H_{E(i)}^{(1)} \cos(\phi_i - \phi_j) \\ &\quad - H_{E(i)}^{(2)} \cos^2(\phi_i - \phi_j) \end{aligned} \quad (29)$$

$$H_{ii}^{\theta\phi} = H_{ii}^{\phi\theta} = 0 \quad (30)$$

$$\frac{1}{M_{si} V} H_{ij}^{\theta\theta} = -2\lambda M_{sj} + H_{E(i)}^{(1)} + H_{E(i)}^{(2)} \cos(\phi_i - \phi_j) \quad (31)$$

$$\frac{1}{M_{si} V} H_{ij}^{\phi\phi} = M_{sj} \lambda 2 \cos(\phi_i - \phi_j) + H_{E(i)}^{(1)} \cos(\phi_i - \phi_j) + H_{E(i)}^{(2)} \cos(2(\phi_i - \phi_j)) \quad (32)$$

$$H_{ij}^{\theta\phi} = H_{ij}^{\phi\theta} = 0 \quad (33)$$

Physically  $\frac{1}{M_{si} V_i} H_{ij}^{kl}$  gives the contribution of the  $l^{th}$  component of the oscillating magnetisation of the  $j^{th}$  layer to the microwave field in the  $k^{th}$  direction in the  $i^{th}$  layer.

To simulate the resonance frequencies at a given external magnetic field, first we find the equilibrium directions of the two magnetic moments at that field,  $\phi_A$  and  $\phi_B$ , by numerically solving the LLG equation with  $\alpha \neq 0$  until the two magnetisations relax into local minima in energy (23). Then, the eigenvalue equation (21) is solved to find the frequencies of the modes.

## 5 Introduction to group theory

Group theory is a powerful mathematical tool that is widely applied across the physical sciences. However, many non-specialists will be unfamiliar with its use and application to physical problems. The following section serves as a brief introduction to the basic principles and intends to illustrate how group theory can be used to obtain insights into the behaviour of physical systems. Interested readers should refer to references such as [10] for a more detailed discussion.

To the physicist, group theory is associated with the study of the symmetries of physical systems, where the physical system in interest can typically be modelled by a linear eigenvalue equation with the usual form:

$$A\mathbf{x}_i = \lambda_i \mathbf{x}_i \quad (34)$$

where  $A$  is some linear operator,  $\lambda_i$  is a scalar, and  $\mathbf{x}_i$  is a vector representing the dynamics of the system under study. It is important that  $A$  is Hermitian, so the collection of eigenvectors inherit the following properties:

1. They form a complete basis
2. They are orthogonal under the standard inner product

In our case, the eigenvectors are the mathematical representation of the oscillation modes of a SAF. As discussed in the main text, the LLG equation does not have the form given in (34) but can be cast into a related form where properties 1. and 2. still apply, except that they are orthogonal under a *modified* inner product. A symmetry transformation is straightforwardly defined as any physical transformation that leaves the system under consideration unchanged (accounting for any indistinguishability that may be present). If the symmetry transformation for the system modelled by (34) is represented by the matrix  $R$ , then it must be that  $R$  commutes with  $A$ :

$$RAR^{-1} = A \rightarrow [R, A] = 0 \quad (35)$$

By applying  $R$  to (34), we see that  $R\mathbf{x}_i$  must also be a solution with an identical eigenvalue. We can now gather all symmetry operations into a collection, equipped with some operator that allows us to combine them which we will denote as  $\times$ , and ask how each eigenvector is affected by each symmetry operation. Such a collection is a *group* if it satisfies the following four conditions:

1. If  $R$  and  $M$  are two elements of the group with  $R \times M = G$ , then  $G$  must also be an element of the group for all  $R$  and  $M$ ;
2. Associativity is satisfied, i.e.  $R \times (M \times G) = (R \times M) \times G$ ;
3. The identity element  $E$  is a member of the group;
4. For every element in the group  $R$ , its inverse,  $R^{-1}$  is also in the group, with  $R \times R^{-1} = E$ .

Symmetry elements in a physical system can be faithfully represented as matrices and their repeated application obeys the laws of matrix multiplication, so associativity is inherited from the associativity of matrix multiplication. From the same definition of symmetry operation as an operation that leaves the system unchanged, the identity is in our collection. Finally, it follows from (35) that if  $R$  is a symmetry element, then so must be  $R^{-1}$ . Having established that the collection of symmetry elements forms a group, we must now consider how these elements interact with our eigenvectors. If there is only one eigenvector for a specific eigenvalue, then every symmetry operation must transform it back into itself, i.e.  $R\mathbf{x}_i = \mathbf{x}_i$ . However, if there are multiple states corresponding to the same eigenvalue, then a symmetry operation will transform the eigenvectors into a linear combination of one another. For example, let's consider to states  $\mathbf{u}$  and  $\mathbf{v}$ , which have degenerate eigenvalue  $\lambda$ , and assume that the symmetry operations  $R$  and  $M$  transform them in the following way:

$$\begin{aligned} R\mathbf{u} &= a\mathbf{u} + b\mathbf{v} & R\mathbf{v} &= c\mathbf{u} + d\mathbf{v} \\ M\mathbf{u} &= e\mathbf{u} + f\mathbf{v} & M\mathbf{v} &= g\mathbf{u} + h\mathbf{v} \end{aligned} \quad (36)$$

Using the coefficients  $a, b$ , etc. we can form what is known as a representation of the operations  $R$  and  $M$ :

$$\begin{aligned} R &\rightarrow \begin{pmatrix} a & b \\ c & d \end{pmatrix} = \hat{R} \\ M &\rightarrow \begin{pmatrix} e & f \\ g & h \end{pmatrix} = \hat{M} \end{aligned} \quad (37)$$

where we use the notation  $\hat{R}$  and  $\hat{M}$  to refer to the matrix representation of the operation. These coefficients can be easily extracted by taking the inner product with the left-hand side of equations in (36), e.g.  $\mathbf{v}^T R\mathbf{u} = b$ , using the orthogonality and completeness of the set of eigenvectors we demanded from our eigenvalue equation. By repeating the procedure (36) for every symmetry operation, we form

what is known as a *representation* of the group from the eigenvectors, which are then said to *engender* this representation of the group. If there are  $n$  degenerate eigenvectors, then the representation we form in this way will be  $n$ -dimensional. A representation must *preserve the structure of the group*, meaning that, if  $R \times M = G$  the matrix multiplication of the associated representations of  $R$  and  $M$  should produce the representation of  $G$ . It is straightforward to verify this, by successive application of the operators to (34) to generate the representation of the product of the two operators.

In the SAF system under study here. As illustrated in the previous section, by using the method of Smit and Beljers [9, 8] the LLG equation is written in the form:

$$-\omega_{\mu}\mathcal{I}\boldsymbol{\mu} = \gamma\mu_0 H\boldsymbol{\mu} \quad (38)$$

where  $H$  is the Hessian of the free energy of the magnetic system in the space of magnetic configurations and  $\mathcal{I}$  is a matrix that is in general not-positive definite. Hence one may be concerned that self-inner products of the form  $\boldsymbol{\mu}^T \mathcal{I} \boldsymbol{\mu}$  may vanish, rendering the process of extracting the coefficients as above for the case of the standard Hermitian eigenvalue problem, invalid. However, as the Hessian is evaluated at a minimum (the equilibrium positions) in the free energy, it is by definition positive definite. So as long as  $\omega$  does not vanish, by taking the inner product of (38) with  $\boldsymbol{\mu}$ , we see that all eigenvectors of the LLG equation have non-zero norm under the modified inner product, allowing extracting the desired coefficients as required.

We have found the representation engendered by the eigenvectors, but there may be others. It is therefore necessary to partition the representations into two categories, those that are in some sense unique, and those that are not. If we have, for example, a  $n$ -dimensional representation and a  $m$ -dimensional one, we can form a new  $n + m$ -dimensional representation by creating a matrix in block diagonal form with the aforementioned representations along the main diagonal. A representation formed in this way contains no new information than its substituent parts, and so fails our test for uniqueness. If every matrix in the representation is in block diagonal form as above, then we say that it is *reducible*.

It may not be immediately obvious if a representation is reducible or not. We can always generate a new representation from an old one by means of a similarity transformation  $\hat{R} \rightarrow \hat{X}\hat{R}\hat{X}^{-1}$  for every  $R$  in the group (the new set of matrices can be verified to satisfy the 4 axioms and structure preserving requirements). This new representation is merely the old one expressed in a new basis, and so also does not qualify as unique. We consider two representations that are connected by such a similarity transformation to be identical. Thus, if a representation can be transformed by means of a similarity transformation into block diagonal form, then it is also reducible. Having performed this partition of our representations, the ones that remain form a set of "building blocks" for the others and are in some sense the most fundamental representations of our group. We call these representations *irreducible*, and they are the main object of study within group theory.

The representation we obtain from the procedure described in (36)-(37) may be reducible. If it is reducible, we can always find some similarity transformation that casts it into block diagonal as above, and by applying this same transformation to the eigenvectors we obtain a new set of eigenvectors, formed of linear combinations of the old ones, which *transform as the irreducible representations of the group*. We may have multiple sets of eigenvectors transforming as the same irreducible representation independently of one another. Eigenvectors that transform as the same irreducible representation are symmetry bound to be degenerate. Eigenvectors that transform as different representations may be degenerate, but this degeneracy is known as *accidental*, that is it is not a degeneracy mandated by the symmetry of the system. However, group theory still has something to say about these degeneracies. As we will see later, modes that transform according to different versions of the same irreducible representation are not allowed to be degenerate under certain conditions. But, given an initial set of eigenvectors and eigenvalues, we already knew that they were degenerate a-priori. So how does understanding the irreducible representations of the eigenvectors help us analyse the physical problem at hand?

The power of group theory is that having established an initial set of eigenvectors which transform as a known irreducible representation of the group, we can predict and understand their evolution under the application of perturbations on symmetry grounds alone. By applying a perturbation, we will typically lower the symmetry of the system, that is the new symmetry group will consist of the old one minus some elements. Such a group is a sub-group of the original group. The irreducible representations of the old, larger group must still be a representation of the new, smaller group. However, they may not in general be irreducible. To see this, imagine we can find a similarity transformation  $\hat{X}$  that casts all the matrices in our representation into block diagonal form except for one, which we will call  $\hat{T}$ . If

we form a new group by removing  $\hat{T}$  as an element, then the impediment to  $\hat{X}$  block-diagonalising the representation has been removed and the representation is now reducible.

If a representation is made reducible by a lowering of symmetry, then it can be written in block diagonal form composed of multiple irreducible representations of the new group. By calculating this decomposition, we can predict how the degeneracies of the eigenvectors will be affected by the perturbation. For example, suppose we have 3 eigenvectors that transform as a 3-dimensional irreducible representation. Suppose that under a suitable perturbation this representation is reduced to a 2-dimensional and a 1-dimensional irreducible representations. Then one of the eigenvectors will become split off from the other two whose eigenvalues will remain degenerate. We note that this is entirely a consequence of the symmetry of the system and can be calculated from knowledge of the group alone, entirely independently of any physical context or equation.

Synthetic antiferromagnets offer a clear example of this in practice. When applying a magnetic field along the easy-axis below the spin-flop field, even though the magnetic configuration remains unchanged, the application of an external field introduces a preferred direction which lowers the combined system symmetry. Consequently, the modes, which at zero field transform as a 2D irreducible representation of the full group and hence are degenerate, are split apart as the 2D representation of the full group is decomposed into two 1-dimensional irreducible representations of the new lower symmetry group.

Once the irreducible representations associated to each mode have been determined, it is straightforward to determine whether or not the modes are allowed to cross. According to the Wigner-von Neumann avoided crossing theorem [11], two modes can only cross if they transform according to different irreducible representations. Note, the degeneracy at the crossing point is therefore accidental.

## References

- [1] L. Liu, T. Moriyama, D. C. Ralph, and R. A. Buhrman, “Spin-Torque Ferromagnetic Resonance Induced by the Spin Hall Effect,” *Phys. Rev. Lett.*, vol. 106, p. 036601, jan 2011.
- [2] L. D. Landau, J. S. Bell, M. J. Kearsley, L. P. Pitaevskii, E. M. Lifshitz, and J. B. Sykes, *Electrodynamics of Continuous Media. COURSE OF THEORETICAL PHYSICS*, Elsevier Science, 2013.
- [3] T. L. Gilbert, “A Lagrangian formulation of the gyromagnetic equation of the magnetisation field,” *Phys. Rev.*, vol. 100, p. 1243, 1955.
- [4] C. Kittel, “On the Theory of Ferromagnetic Resonance Absorption,” *Phys. Rev.*, vol. 73, no. 155, 1948.
- [5] A. G. Gurevic and G. A. Melkov, *Magnetization Oscillations and Waves*. London: CRC Press, 1st editio ed., 1996.
- [6] R. Lavrijsen, A. Fernandez-Pacheco, D. Petit, R. Mansell, J. H. Lee, and R. P. Cowburn, “Tuning the interlayer exchange coupling between single perpendicularly magnetized CoFeB layers,” *Appl. Phys. Lett.*, vol. 100, no. 5, p. 52411, 2012.
- [7] A. J. Newell, D. J. Dunlop, and W. Williams, “A generalization of the demagnetizing tensor for nonuniform magnetization,” *J. Geophys. Res.*, vol. 98, no. B6, p. 9551, 1993.
- [8] M. Grimsditch, L. Giovannini, F. Montoncello, F. Nizzoli, G. K. Leaf, and H. G. Kaper, “Magnetic normal modes in ferromagnetic nanoparticles: A dynamical matrix approach,” *Phys. Rev. B*, vol. 70, no. 054409, pp. 1–7, 2004.
- [9] J. Smit and H. G. Beljers, “Ferromagnetic Resonance absorption in BaFe<sub>12</sub>O<sub>19</sub> a highly anisotropic crystal,” *Philips Res. Rep.*, vol. 10, no. 113, 1955.
- [10] M. Dresselhaus, G. Dresselhaus, and A. Jorio, *Group Theory: Application to the Physics of Condensed Matter*. Springer, 1 ed., 2008.
- [11] P. Wigner, *The Collected Works of Eugene Paul Wigner*. Berlin: Springer-Verlag Berlin Heidelberg, 1 ed., 1993.
